# Supplementary material for: Harnessing the power of longitudinal medical imaging for eye disease prognosis using Transformer-based sequence modeling
Source: arXiv:2405.08780 source file (2024-07-30)
Supplement: Supplementary file 1 [file LTSA_Supplement.pdf]

**Supplementary Table 1 | Full late AMD prognosis results.**

| t |          | $\Delta t=1$                | $\Delta t=2$                | $\Delta t=5$                | $\Delta t=8$                |
|---|----------|-----------------------------|-----------------------------|-----------------------------|-----------------------------|
| 1 | Baseline | 0.818 (0.771, 0.862)        | 0.825 (0.787, 0.861)        | 0.848 (0.818, 0.875)        | 0.858 (0.834, 0.881)        |
|   | LTSA     | <b>0.823 (0.775, 0.863)</b> | <b>0.836 (0.802, 0.868)</b> | <b>0.851 (0.826, 0.874)</b> | <b>0.854 (0.832, 0.876)</b> |
| 2 | Baseline | 0.897 (0.862, 0.927)        | 0.886 (0.858, 0.911)        | 0.884 (0.860, 0.907)        | 0.883 (0.860, 0.904)        |
|   | LTSA     | <b>0.938 (0.918, 0.956)</b> | <b>0.923 (0.903, 0.940)</b> | <b>0.913 (0.895, 0.930)</b> | <b>0.907 (0.891, 0.921)</b> |
| 3 | Baseline | 0.908 (0.885, 0.929)        | 0.896 (0.873, 0.917)        | 0.883 (0.862, 0.903)        | 0.877 (0.858, 0.897)        |
|   | LTSA     | <b>0.943 (0.928, 0.957)</b> | <b>0.927 (0.911, 0.942)</b> | <b>0.905 (0.890, 0.920)</b> | <b>0.897 (0.882, 0.911)</b> |
| 5 | Baseline | 0.930 (0.914, 0.944)        | 0.910 (0.894, 0.926)        | 0.888 (0.870, 0.905)        | 0.878 (0.858, 0.896)        |
|   | LTSA     | <b>0.959 (0.951, 0.967)</b> | <b>0.936 (0.924, 0.947)</b> | <b>0.917 (0.905, 0.929)</b> | <b>0.906 (0.893, 0.919)</b> |
| 8 | Baseline | 0.919 (0.905, 0.931)        | 0.911 (0.897, 0.925)        | 0.892 (0.876, 0.908)        | 0.892 (0.875, 0.909)        |
|   | LTSA     | <b>0.939 (0.929, 0.948)</b> | <b>0.934 (0.924, 0.943)</b> | <b>0.920 (0.908, 0.931)</b> | <b>0.919 (0.908, 0.931)</b> |

Detailed quantitative late AMD prognosis results by time-dependent concordance index  $C(t, \Delta t)$  for various values of prediction time  $t$  and evaluation time  $\Delta t$ . Presented is the mean  $C(t, \Delta t)$  from 1,000 bootstrap samples of the test set, with 95% bootstrapped confidence intervals in parentheses. Results from our proposed LTSA appear in boldface with a grey background, while the baseline results appear in standard font with a white background. LTSA = Longitudinal Transformer for Survival Analysis. AMD – Age-related Macular Degeneration.

**Supplementary Table 2 | Full POAG prognosis results.**

| t |          | $\Delta t=1$                | $\Delta t=2$                | $\Delta t=5$                | $\Delta t=8$                |
|---|----------|-----------------------------|-----------------------------|-----------------------------|-----------------------------|
| 1 | Baseline | 0.881 (0.693, 0.991)        | 0.892 (0.751, 0.981)        | 0.852 (0.785, 0.910)        | 0.860 (0.815, 0.904)        |
|   | LTSA     | <b>0.891 (0.764, 0.996)</b> | <b>0.898 (0.817, 0.972)</b> | <b>0.861 (0.800, 0.920)</b> | <b>0.867 (0.817, 0.911)</b> |
| 2 | Baseline | 0.917 (0.803, 0.988)        | 0.830 (0.660, 0.972)        | 0.783 (0.706, 0.854)        | 0.819 (0.765, 0.868)        |
|   | LTSA     | <b>0.925 (0.859, 0.990)</b> | <b>0.913 (0.863, 0.957)</b> | <b>0.870 (0.821, 0.915)</b> | <b>0.902 (0.872, 0.931)</b> |
| 3 | Baseline | 0.858 (0.746, 0.970)        | 0.848 (0.777, 0.913)        | 0.801 (0.732, 0.865)        | 0.837 (0.789, 0.884)        |
|   | LTSA     | <b>0.923 (0.879, 0.962)</b> | <b>0.902 (0.856, 0.945)</b> | <b>0.885 (0.846, 0.920)</b> | <b>0.914 (0.886, 0.939)</b> |
| 5 | Baseline | 0.894 (0.852, 0.933)        | 0.886 (0.848, 0.921)        | 0.892 (0.863, 0.919)        | 0.896 (0.871, 0.919)        |
|   | LTSA     | <b>0.920 (0.893, 0.946)</b> | <b>0.903 (0.868, 0.934)</b> | <b>0.924 (0.901, 0.944)</b> | <b>0.933 (0.914, 0.952)</b> |
| 8 | Baseline | 0.887 (0.842, 0.927)        | 0.901 (0.865, 0.931)        | 0.899 (0.863, 0.928)        | 0.898 (0.863, 0.928)        |
|   | LTSA     | <b>0.937 (0.918, 0.954)</b> | <b>0.944 (0.928, 0.958)</b> | <b>0.950 (0.936, 0.962)</b> | <b>0.949 (0.935, 0.962)</b> |

Detailed quantitative POAG prognosis results by time-dependent concordance index  $C(t, \Delta t)$  for various values of prediction time  $t$  and evaluation time  $\Delta t$ . Presented is the mean  $C(t, \Delta t)$  from 1,000 bootstrap samples of the test set, with 95% bootstrapped confidence intervals in parentheses. Results from our proposed LTSA appear in boldface with a grey background, while the baseline results appear in standard font with a white background. LTSA = Longitudinal Transformer for Survival Analysis. AMD – Age-related Macular Degeneration.

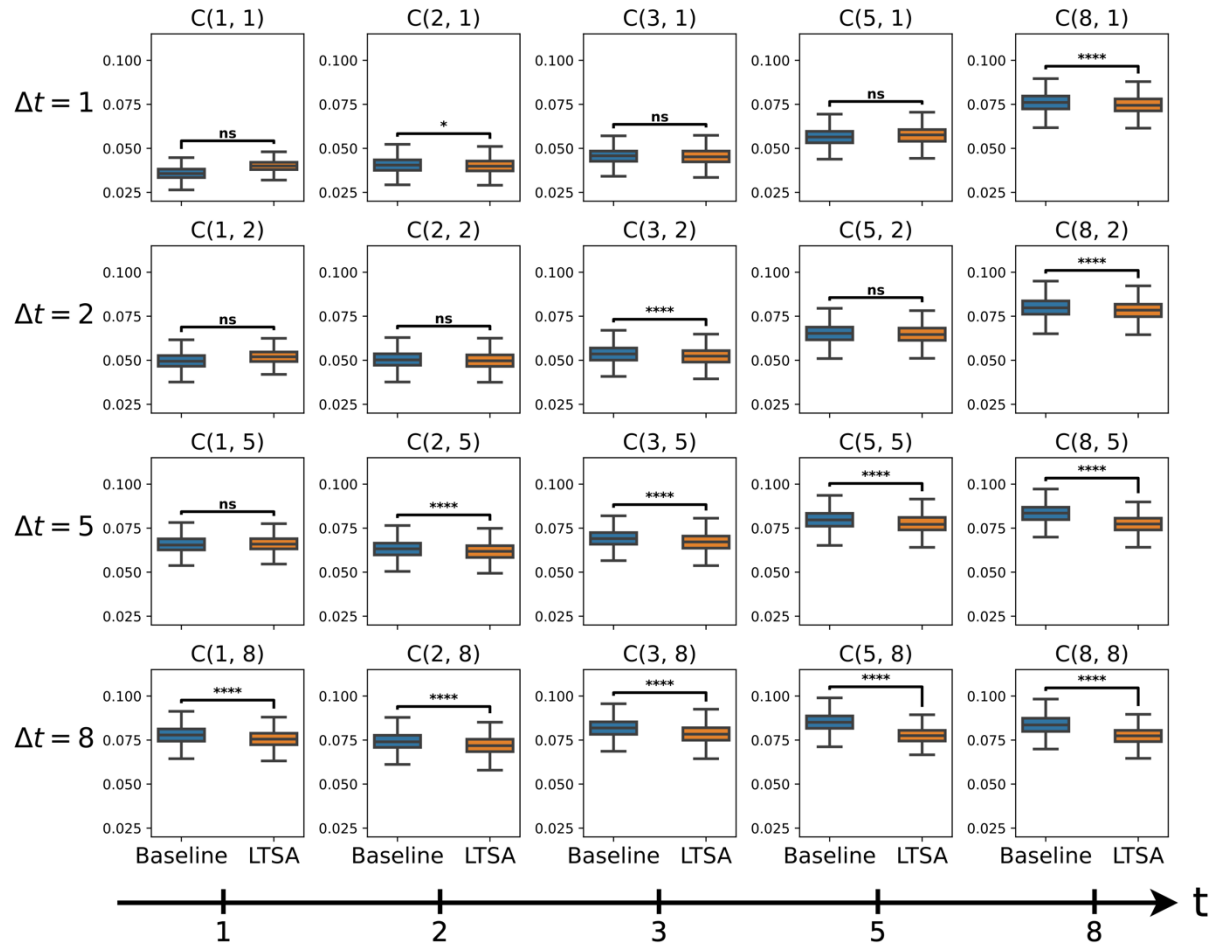

**Supplementary Figure 1 | Auxiliary late AMD prognosis results.** Time-dependent Brier score  $B(t, \Delta t)$  for various values of prediction time  $t$  and evaluation time  $\Delta t$  comparing the single-image baseline model (blue) to LTSA, which incorporates all prior visits (orange). Box plots depict the values computed from 1,000 bootstrap samples of the test set (center line = median, box = IQR, whiskers = 1.5x the IQR from the box). Significance levels are determined from Bonferroni-adjusted  $P$ -values as follows: \*\*\*\* =  $P \leq 0.0001$ , \*\*\* =  $P \leq 0.001$ , \*\* =  $P \leq 0.01$ , \* =  $P \leq 0.05$ , ns = no significant difference. AMD = age-related macular degeneration; IQR = interquartile range.

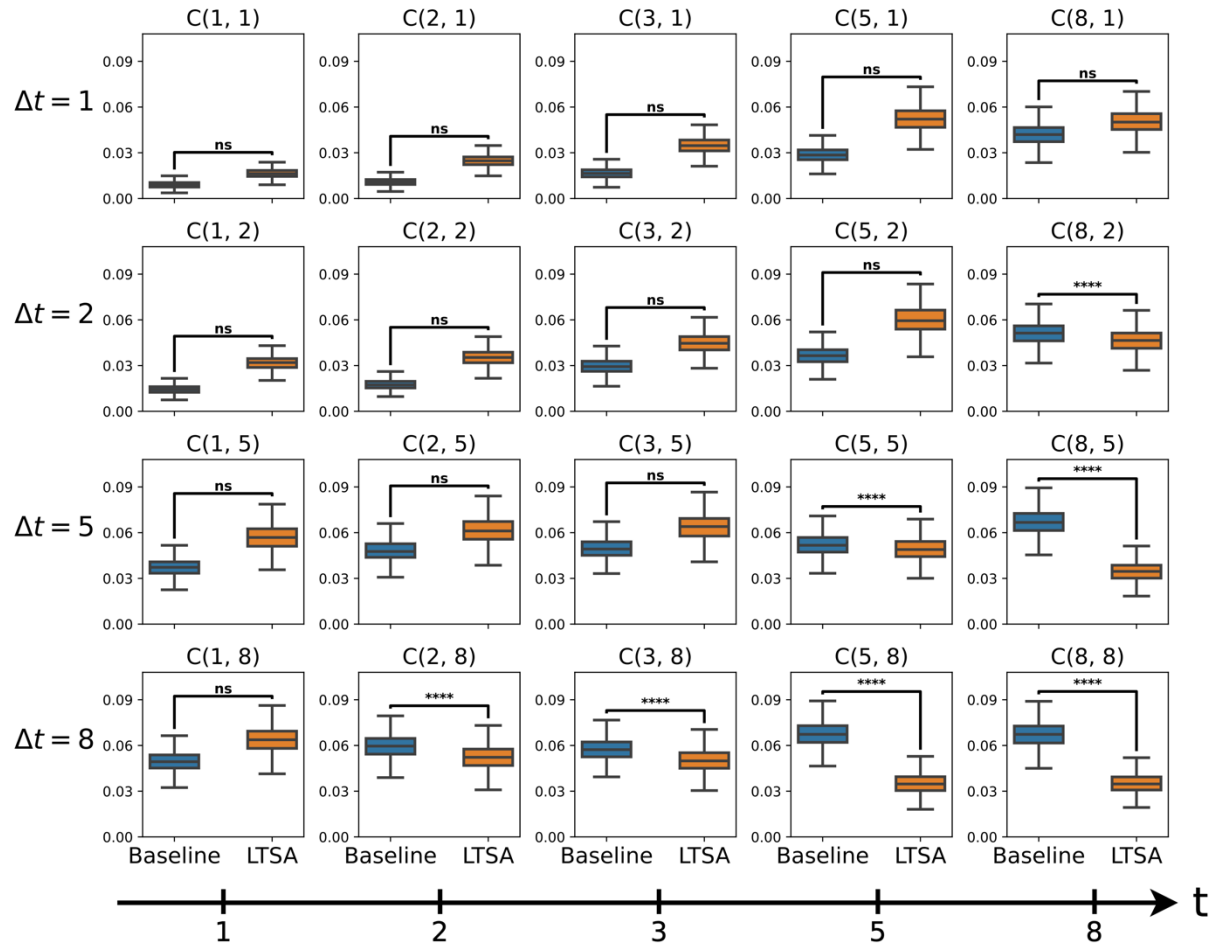

**Supplementary Figure 2 | Auxiliary POAG prognosis results.** Time-dependent Brier score  $B(t, \Delta t)$  for various values of prediction time  $t$  and evaluation time  $\Delta t$  comparing the single-image baseline model (blue) to LTSA, which incorporates all prior visits (orange). Box plots depict the values computed from 1,000 bootstrap samples of the test set (center line = median, box = IQR, whiskers = 1.5x the IQR from the box). Significance levels are determined from Bonferroni-adjusted  $P$ -values as follows: \*\*\*\* =  $P \leq 0.0001$ , \*\*\* =  $P \leq 0.001$ , \*\* =  $P \leq 0.01$ , \* =  $P \leq 0.05$ , ns = no significant difference. IQR = interquartile range; POAG = primary open-angle glaucoma.

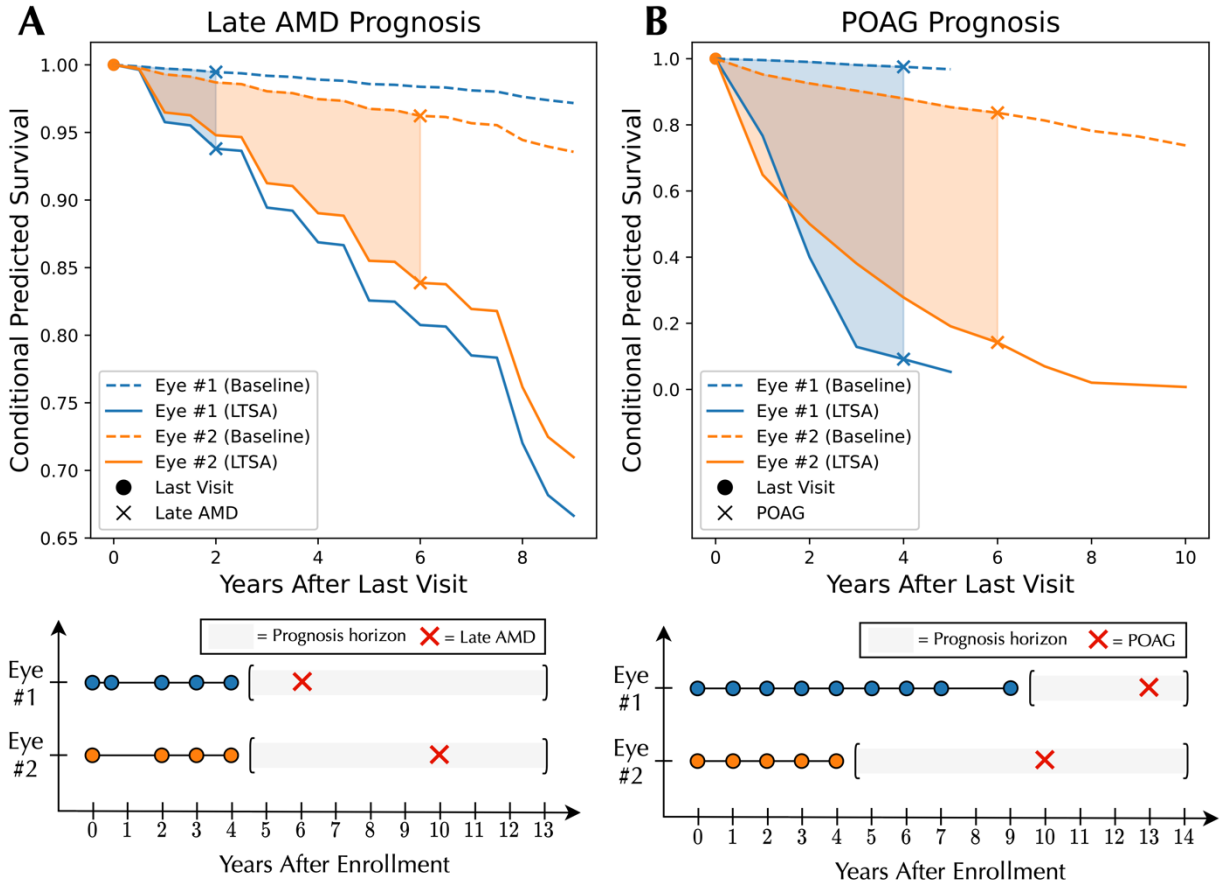

**Supplementary Figure 3 | Longitudinal modeling better captures eye disease risk.** Predicted conditional survival curves comparing the baseline model (only using last available visit) and our longitudinal model (using all available visits) prognoses for two unique eyes in the AREDS test set (**A**) and two unique eyes in the OHTS test set (**B**). Visualizations below each panel depict the longitudinal visit times, event times, and prognosis horizons for each eye in panels **A** and **B**, respectively. AMD = age-related macular degeneration. AREDS = Age-Related Eye Disease Study; OHTS = Ocular Hypertension Treatment Study; POAG = primary open-angle glaucoma.
